# Supplementary material for: Syntax-augmented Multilingual BERT for Cross-lingual Transfer
Source: arXiv:2106.02134 source file (2021-06-03)
Supplement: Supplementary file 1 [file conll.tex]

% \begin{table*}[t]
% 	\centering
% % 	\resizebox{\linewidth}{!}{%
% % 	\small
% 	\begin{tabular}{c | c | @{\hskip 0.15in}c@{\hskip 0.15in} | c}
% 		\hline
% 		\multirow{2}{*}{Lang} & \multicolumn{3}{c}{mBERT} \\ 
% 		\cline{2-4}
% 		& \citeauthor{liang2020xglue} & (ours) & + Syn. \\
% 		\hline
% 		%=====
%         EN	& 90.6 & 90.7 & 90.6 \\
%         DE	& 69.2 & 68.4 & 69.1 \\
%         ES	& 75.4 & 73.4 & 73.6 \\
%         NL	& 77.9 & 77.6 & 78.5 \\ \hline
%         Average	& 78.2 & 77.5 & 78.0  \\
% 		%===========
% 		\hline
% 	\end{tabular}
% % }
% \caption{
% Cross-lingual transfer results (on test set) for CoNLL 2002 \cite{tjong-kim-sang-2002-introduction} and 2003 \cite{tjong-kim-sang-de-meulder-2003-introduction} NER datasets.
% } 
% \label{table:panx} 
% % \vspace{-1em}
% \end{table*}

\begin{table*}[t]
\centering
% 	\resizebox{\linewidth}{!}{%
% 	\small
\begin{tabular}{l|c c c c|c}
\hline
models & en & de & es & nl & avg \\
\hline
\citet{liang2020xglue} & 90.6 & 69.2 & 75.4 & 77.9 & 78.2  \\
mBERT (ours) & 90.7 & 68.4 & 73.4 & 77.6 & 77.5 \\ 
mBERT+Syn. & 90.6 & 69.1 & 73.6 & 78.5 & 78.0 \\
\hline
\end{tabular}
% }
\caption{
Cross-lingual transfer results (on test set) for CoNLL 2002 \cite{tjong-kim-sang-2002-introduction} and 2003 \cite{tjong-kim-sang-de-meulder-2003-introduction} NER datasets.
} 
\label{table:conll} 
% \vspace{-1em}
\end{table*}
