# Supplementary material for: Syntax-augmented Multilingual BERT for Cross-lingual Transfer
Source: arXiv:2106.02134 source file (2021-06-03)
Supplement: Supplementary file 2 [file mlqa_gxlt.tex]

% \begin{table}[!ht]
% \centering
% % \resizebox{\linewidth}{!}{%
% % \small
% \begin{tabular}{l| c c c c c c c}
% \hline
% q/c	&	en	&	es	&	de	&	ar	&	hi	&	vi	&	zh	\\ \hline
% en	&	0	&	-0.2	&	0.3	&	0.4	&	0.9	&	0.6	&	1.1	\\ 
% es	&	\cellcolor{lgray}4.1	&	2	&	\cellcolor{lgray}3.5	&	\cellcolor{lgray}5.4	&	\cellcolor{lgray}5.3	&	\cellcolor{lgray}7.3	&	\cellcolor{lgray}7.6	\\
% de	&	\cellcolor{lgray}3.5	&	\cellcolor{lgray}2.8	&	1.8	&	\cellcolor{lgray}4	&	\cellcolor{lgray}2.9	&	\cellcolor{lgray}4	&	\cellcolor{lgray}5	\\
% de	&	1.8	&	2.4	&	1.1	&	1.6	&	-0.1	&	\cellcolor{lgray}6.2	&	\cellcolor{lgray}4.4	\\
% hi	&	1	&	1.8	&	0.5	&	0.2	&	-0.8	&	-0.6	&	1	\\
% vi	&	\cellcolor{lgray}5.6	&	\cellcolor{lgray}4.5	&	\cellcolor{lgray}5.5	&	\cellcolor{lgray}6.9	&	\cellcolor{lgray}4.2	&	\cellcolor{lgray}2.8	&	\cellcolor{lgray}5.5	\\
% zh	&	\cellcolor{lgray}3.8	&	\cellcolor{lgray}3.3	&	\cellcolor{lgray}4.4	&	2.4	&	0.9	&	\cellcolor{lgray}5.4	&	2.3	\\
% \hline
% \end{tabular}
% % }
% % \vspace{-2mm}
% \caption{
% F1 score difference for generalized cross-lingual transfer for MLQA.  
% Columns show context language, rows show question language.
% The gray cells have a value $>=$ 2.8 (average difference).
% }
% % }
% \label{table:mlqa_xling}
% % \vspace{-2mm}
% \end{table}

%%%%%%%%%%%%%%%%%%%%%%%%%%%%%%%%%%%%%%%%%%%%%%%%%%%%%%%%%%%%%%%%
\begin{table}[!ht]
\centering
% \resizebox{\linewidth}{!}{%
% \small
\begin{tabular}{l| c c c c c c c}
\hline
q/c	&	en	&	es	&	de	&	ar	&	hi	&	vi	&	zh	\\ \hline
en	&	-	&	-0.2	&	0.3	&	0.4	&	0.9	&	0.6	&	1.1	\\ 
es	&	\cellcolor{lgray}4.1	&	-	&	\cellcolor{lgray}3.5	&	\cellcolor{lgray}5.4	&	\cellcolor{lgray}5.3	&	\cellcolor{lgray}7.3	&	\cellcolor{lgray}7.6	\\
de	&	\cellcolor{lgray}3.5	&	2.8	&	-	&	\cellcolor{lgray}4.0	&	2.9	&	\cellcolor{lgray}4.0	&	\cellcolor{lgray}5.0	\\
de	&	1.8	&	2.4	&	1.1	&	-	&	-0.1	&	\cellcolor{lgray}6.2	&	\cellcolor{lgray}4.4	\\
hi	&	1.0	&	1.8	&	0.5	&	0.2	&	-	&	-0.6	&	1.0	\\
vi	&	\cellcolor{lgray}5.6	&	\cellcolor{lgray}4.5	&	\cellcolor{lgray}5.5	&	\cellcolor{lgray}6.9	&	\cellcolor{lgray}4.2	&	-	&	\cellcolor{lgray}5.5	\\
zh	&	\cellcolor{lgray}3.8	&	\cellcolor{lgray}3.3	&	\cellcolor{lgray}4.4	&	2.4	&	0.9	&	\cellcolor{lgray}5.4	&	-	\\
\hline
\end{tabular}
% }
% \vspace{-2mm}
\caption{
The cross-lingual transfer performance (F1 score) difference between syntax-augmented mBERT and mBERT on the MLQA dataset in the \emph{generalized} setting.
Columns show context language, rows show question language.
The gray cells have a value $\geq$ 3.1 (average difference).
}
% }
\label{table:mlqa_xling}
% \vspace{-2mm}
\end{table}
