# Supplementary material for: Syntax-augmented Multilingual BERT for Cross-lingual Transfer
Source: arXiv:2106.02134 source file (2021-06-03)
Supplement: Supplementary file 3 [file overall.tex]

%%%%%%%%%%%%%%%%%%%%%%%%%%%%%%%%%%%%%%%%%%%%%%%%%%%%%%%%%%%%%%%%
\begin{table*}[!ht]
\centering
\resizebox{\linewidth}{!}{%
% \small
\begin{tabular}{l|c@{\hskip 0.1in} c|c@{\hskip 0.1in} c|c@{\hskip 0.1in} c|c@{\hskip 0.1in} c}
\hline
Model & XNLI & PAWS-X & Wikiann & CoNLL & MLQA & XQuAD & mTOP & mATIS++ \\
\hline 
mBERT & 67.5$^\ast$ & 82.0$^\ast$ & 69.5$^\ast$ & 78.2$^\dagger$ & 57.7/41.6$^\star$ & 66.7/51.0$^\ast$ & - & - \\
mBERT (ours) & 67.5 & 82.9 & 68.5 & 77.8 & 58.9/40.5 & 63.4/46.9 & 39.6 & 32.9 \\
mBERT+Syn. & {\bf 68.5} & {\bf 84.3} & 69.0 & 78.0 &  {\bf 60.3}/{\bf 42.2} & 64.2/48.4 & {\bf 41.4} & {\bf 33.6} \\
\hline
\end{tabular}
}
% \vspace{-2mm}
\caption{
Average zero-shot cross-lingual performance on the evaluation datasets.
$^\ast$, $^\dagger$, and $^\star$  indicates the results are reported from \citet{hu2020xtreme}, \citet{liang2020xglue}, and \citet{lewis-etal-2020-mlqa}, respectively.
``(ours)'' indicates the result we produce on the pre-processed datasets and we consider it as the \emph{baseline} for syntax-augmented mBERT throughout all the experiments.
Except for the QA datasets, all our results are averaged over three different seeds. 
}
\label{table:overall}
% \vspace{-2mm}
\end{table*}
