# Supplementary material for: Syntax-augmented Multilingual BERT for Cross-lingual Transfer
Source: arXiv:2106.02134 source file (2021-06-03)
Supplement: Supplementary file 4 [file panx.tex]

% \begin{table}[t]
% 	\centering
% % 	\resizebox{\linewidth}{!}{%
% % 	\small
% 	\begin{tabular}{c | c | @{\hskip 0.15in}c@{\hskip 0.15in} | c}
% 		\hline
% 		\multirow{2}{*}{Lang} & \multicolumn{3}{c}{mBERT} \\ 
% 		\cline{2-4}
% 		& \citeauthor{hu2020xtreme} & (ours) & + Syn. \\
% 		\hline
% 		%=====
%         EN	&	85.2	&	83.6	&	84.4	\\ \hline
%         AR	&	41.1	&	38.8	&	40.0	\\
%         BG	&	77.0	&	77.0	&	77.0	\\
%         DE	&	78.0	&	76.0	&	77.0	\\
%         EL	&	72.5	&	70.4	&	71.5	\\
%         ES	&	77.4	&	74.7	&	76.1	\\
%         FR	&	79.6	&	78.9	&	79.3	\\
%         HI	&	65.0	&	63.4	&	64.2	\\
%         KO	&	59.6	&	58.9	&	59.3	\\
%         NL	&	81.8	&	81.9	&	81.9	\\
%         PT	&	80.8	&	78.7	&	79.0	\\
%         RU	&	64.0	&	63.5	&	63.8	\\
%         TR	&	71.8	&	70.9	&	71.4	\\
%         UR	&	36.9	&	37.7	&	37.3	\\
%         VI	&	71.8	&	73.5	&	72.7	\\
%         Average	&	69.5	&	68.5	&	69	\\
% 		%===========
% 		\hline
% 	\end{tabular}
% % }
% \caption{
% Cross-lingual transfer results (F1 score) for named entity recognition (on test set) using Wikiann dataset \cite{pan-etal-2017-cross} across 15 languages.
% } 
% \label{table:panx} 
% % \vspace{-1em}
% \end{table}

%%%%%%%%%%%%%%%%%%%%%%%%%%%%%%%%%%%%%%%%%%%%%%%%%%%%%%%%%%%%%%%%
\begin{table*}[!ht]
\centering
\resizebox{\linewidth}{!}{%
% \small
\begin{tabular}{l@{\hskip 0.05in}|@{\hskip 0.05in}c@{\hskip 0.1in} c@{\hskip 0.1in} c@{\hskip 0.1in} c@{\hskip 0.1in} c@{\hskip 0.1in} c@{\hskip 0.1in} c@{\hskip 0.1in} c@{\hskip 0.1in} c@{\hskip 0.1in} c@{\hskip 0.1in} c@{\hskip 0.1in} c@{\hskip 0.1in} c@{\hskip 0.1in} c@{\hskip 0.1in} c@{\hskip 0.05in}|@{\hskip 0.05in}c@{\hskip 0.05in}}
\hline
models & en & ar & bg & de & el & es & fr & hi & ko & nl & pt & ru & tr & ur & vi & avg \\
\hline
\citet{hu2020xtreme} &  85.2 & 41.1 & 77.0 & 78.0 & 72.5& 77.4 & 79.6& 65.0 & 59.6 & 81.8 & 80.8 & 64.0 & 71.8 & 36.9 & 71.8 & 69.5 \\
mBERT (ours) &  83.6 & 38.8 & 77.0 & 76.0 & 70.4 & 74.7 & 78.9 & 63.4 & 58.9 & 81.9 & 78.7 & 63.5 & 70.9 & 37.7 & 73.5 & 68.5\\
mBERT+Syn. & 84.4 & 40.0 & 77.0 & 77.0 & 71.5 & 76.1 & 79.3 & 64.2 & 59.3 & 81.9 & 79.0 & 63.8 & 71.4 & 37.3 & 72.7 & 69.0 \\
\hline
\end{tabular}
}
% \vspace{-2mm}
\caption{
Cross-lingual transfer results (F1 score) for named entity recognition (on test set) using Wikiann dataset \cite{pan-etal-2017-cross} across 15 languages.
}
% }
\label{table:panx}
% \vspace{-2mm}
\end{table*}
