# Supplementary material for: Syntax-augmented Multilingual BERT for Cross-lingual Transfer
Source: arXiv:2106.02134 source file (2021-06-03)
Supplement: Supplementary file 5 [file pawsx.tex]

%%%%%%%%%%%%%%%%%%%%%%%%%%%%%%%%%%%%%%%%%%%%%%%%%%%%%%%%%%%%%%%%
\begin{table*}[!ht]
\centering
% \resizebox{\linewidth}{!}{%
% \small
\begin{tabular}{l|c c c c c c c |c}
\hline
models & en & de & es & fr & ja & ko & zh & avg \\
\hline
\citet{hu2020xtreme} & 94.0 & 85.7 & 87.4 & 87.0 & 73.0 & 69.6 & 77.0 & 82.0 \\
mBERT (ours) & 93.9 & 85.7 & 88.4 & 87.6 & 73.1 & 73.6 & 78.0 & 82.9 \\ 
mBERT+Syn. & 94.0 & 85.9 & 89.1 & 88.2 & 75.8 & 76.3 & 80.7 & 84.3 \\
\hline
\end{tabular}
% }
% \vspace{-2mm}
\caption{
Zero-shot cross-lingual PAWS-X accuracy scores for each language. 
% [1] indicates the results are reported from \cite{hu2020xtreme}. 
% All our results are averaged over three different seeds.
}
% }
\label{table:pawsx_result}
% \vspace{-2mm}
\end{table*}
