# Supplementary material for: Syntax-augmented Multilingual BERT for Cross-lingual Transfer
Source: arXiv:2106.02134 source file (2021-06-03)
Supplement: Supplementary file 6 [file xnli.tex]

%%%%%%%%%%%%%%%%%%%%%%%%%%%%%%%%%%%%%%%%%%%%%%%%%%%%%%%%%%%%%%%%
\begin{table*}[!ht]
\centering
\resizebox{\linewidth}{!}{%
% \small
\begin{tabular}{l|c@{\hskip 0.1in} c@{\hskip 0.1in} c@{\hskip 0.1in} c@{\hskip 0.1in} c@{\hskip 0.1in} c@{\hskip 0.1in} c@{\hskip 0.1in} c@{\hskip 0.1in} c@{\hskip 0.1in} c@{\hskip 0.1in} c@{\hskip 0.1in} c@{\hskip 0.1in} c|c}
\hline
models & en & ar & bg & de & el & es & fr & hi & ru & tr & ur & vi & zh & avg \\
\hline
\citet{hu2020xtreme} & 80.8 & 64.3 & 68.0 & 70.0 & 65.3 & 73.5 & 73.4 & 58.9 & 67.8 & 60.9 & 57.2 & 69.3 & 67.8 & 67.5 \\
mBERT (ours) & 81.8 & 63.8 & 68.0 & 70.7 & 65.4 & 73.8 & 72.4 & 59.3 & 68.4 & 60.7 & 56.7 & 68.6 & 67.8 & 67.5 \\
mBERT+Syn. & 81.6 & 65.4 & 69.3 & 70.7 & 66.5 & 74.1 & 73.2 & 60.5 & 68.8 & 62.4 & 58.7 & 69.9 & 69.3 & 68.5 \\
\hline
\end{tabular}
}
% \vspace{-2mm}
\caption{Zero-shot cross-lingual XNLI accuracy scores for each language. We do not consider the Swahili (sw) and Thai (th) languages as UDPipe \cite{straka-strakova-2017-tokenizing} does not support those languages.
% [1] indicates that the results are reported from \cite{hu2020xtreme}.
% All our results are averaged over three different seeds.
}
% }
\label{table:xnli_result}
% \vspace{-2mm}
\end{table*}
