# Supplementary material for: Syntax-augmented Multilingual BERT for Cross-lingual Transfer
Source: arXiv:2106.02134 source file (2021-06-03)
Supplement: Supplementary file 7 [file xquad.tex]

%%%%%%%%%%%%%%%%%%%%%%%%%%%%%%%%%%%%%%%%%%%%%%%%%%%%%%%%%%%%%%%%
\begin{table*}[!ht]
\centering
% \resizebox{\linewidth}{!}{%
% \small
% \begin{tabular}{l|c@{\hskip 0.05in}| c@{\hskip 0.05in}| c@{\hskip 0.05in}| c@{\hskip 0.05in}| c@{\hskip 0.05in}| c@{\hskip 0.05in}| c|c}
\begin{tabular}{l|c c c c c c c c c c|c}
\hline
models & en & es & de & el & ru & tr & ar & vi & zh & hi & avg \\
\hline 
\citet{hu2020xtreme}. & 83.5 & 75.5 & 70.6 & 62.6 & 71.3 & 55.4 & 61.5 & 69.5 & 58.0 & 59.2 & 66.7 \\
% \text{[2]} & 88.9 & 75.5 & 70.6 & 62.6 & 71.3 & 55.4 & 61.5 & 69.5 & 58.0 & 59.2 & 65.0 \\
mBERT (ours) & 84.2 & 71.1 & 68.9 & 60.2 & 68.6 & 48.9 & 54.8 & 64.0 & 57.2 & 55.7 & 63.4 \\ 
mBERT+Syn. & 84.0 & 72.8 & 71.4 & 61.3 & 68.4 & 49.8 & 55.5 & 67.6 & 56.1 & 54.6 & 64.2 \\
\hline
\end{tabular}
% }
% \vspace{-2mm}
\caption{
Zero-shot cross-lingual transfer performance (F1) of mBERT on XQuAD dataset. 
}
% }
\label{table:xquad}
% \vspace{-2mm}
\end{table*}
